# Supplementary material for: Universal Policies to Learn Them All
Source: arXiv:1908.09184 source file (2019-08-24)
Supplement: Supplementary file 1 [file Appendix.tex]

\appendix
\begin{table}[ht]
\centering
\begin{tabular}{l|l|l|l|l|}
\cline{2-5}
 & RL & SM & Street & Pie-in-the-face \\ \hline
\multicolumn{1}{|l|}{ $\alpha$} & 2 & 2 & 2.5 & 4 \\ \hline
\multicolumn{1}{|l|}{$\beta$} & 2 & 1 & 2 & 1 \\ \hline
\end{tabular}
\caption{$\alpha$ and $\beta$ values for the reward function for different scenarios}
\end{table}
\section{Derivation}
\label{appedix:derivation}
Let the objective function of bodyguard $i$ be
\begin{equation}
\label{eq:objfunc}
J(\theta_i)= \mathbb{E}_\pi\left[\displaystyle \sum_t \gamma^t R(s^t, a^t, g)\right]
\end{equation}

Applying the policy gradient theorem by~\cite{Sutton-1998-Book} to~\cref{eq:objfunc}, the objective function is maximized by moving the policy parameters in the direction of the gradient that is given by

\begin{equation}
\label{eq:objfuncgrad}
\nabla J(\theta_i) = \mathbb{E}_\pi\left[\nabla \log \pi \left(a | s, g \right) Q_i^\pi(s, a, g)\right]
\end{equation}

\noindent where $Q_i^\pi(s, a, g)$ is the universal state-action value function approximator. ~\cite{Foerster-2018-AAAI} and~\cite{Lowe-2017-NIPS} have shown that using a centralized critic performs better than using a decentralized critic thus replacing the $Q_i^\pi(s, a, g)$ in~\cref{eq:objfuncgrad} with a centralized critic $Q^\pi(s, a_1, \ldots, a_n, g)$, the updated policy gradient becomes 
\begin{equation}
\label{eq:centeral_critic_grad}
\nabla J(\theta_i) = \mathbb{E}_\pi\left[ \nabla \log \pi \left(a | s, g \right) Q^\pi(s, a_1, \ldots, a_n , g)\right]
\end{equation}

In~\cite{Silver-2014-ICML} have show that the policy gradient can also be written as $\nabla J{\left(\theta\right)}=\mathbb{E}\left[\nabla_{\theta}\pi\left(a|s\right)\nabla_{a}Q^{\pi}\left(s,a\right)|_{a=\pi\left(s\right)}\right]$. By applying the aforementioned trick on~\cref{eq:centeral_critic_grad}, the updated policy gradient can be written as  
\begin{equation}
\label{eq:pol_grad}
\nabla J{\left(\theta_i\right)}=\mathbb{E}_\pi\left[\nabla_{\theta_i}\pi\left(a|s, g\right)\nabla _{a_i}Q^{\pi}\left(s,a_{1},\ldots,a_{N}, g\right)|_{a_i=\pi_i\left(s, g\right)}\right]
\end{equation}

Since all the derivation holds true in case of partial observability of environment, we can replace the state input $s_t$ to the agent at time $t$ with the observation $o_t$ to the agent at time $t$. Then the policy gradient in~\cref{eq:pol_grad} can be written as 

\begin{equation}
\label{eq:pol_grad_upg}
\nabla J{\left(\theta_i\right)}=\mathbb{E}_\pi\left[\nabla_{\theta_i}\pi\left(a|o_i, g\right)\nabla _{a_i}Q^{\pi}\left(s,a_{1},\ldots,a_{N}, g\right)|_{a_i=\pi_i\left(o_i, g\right)}\right]
\end{equation}

\noindent which we refer as multi-agent universal policy gradient.

\section{Network Architecture and Hyperparameters}
Both the actor and the critic networks for all agents consists of 2 hidden layers containing 64 units in each layer. The hidden layers use ReLU activation function while the output layers of both the networks use linear activation function. Both the networks are initialized using Xavier normal initializers.  However,  the output layer of the critics were initialized with zero weights to enable one-step look ahead learning of the critics after each training cycle. Same architecture was used across all the experiments.

Policies for each scenario were trained using different set of parameters while keeping the length of each episode 25 across all experiments. Random Landmark scenario was trained for 8,000 episodes. The other 3 remaining environments were trained for 5000 episodes respectively. The universal policy was trained for 9000 episodes. Minibatches of size 1024 were sampled from replay buffer of size 10$^7$ for each agent and 4 optimization steps were performed on all the critics. We update the target network after every optimization cycle using Polyak Averaging with decay coefficient of 0.99. For Adam optimization algorithm we used learning rate of 0.001 and default values from TensorFlow framework for remaining hyperparameters. Finally the discount factor $\gamma$ was choose to be 0.75 across all experiments.
